# Supplementary material for: InternVideo: General Video Foundation Models via Generative and Discriminative Learning
Source: arXiv:2212.03191 source file (2022-12-07)
Supplement: Supplementary file 1 [file appendix.tex]

% !TeX spellcheck = en_US
%!TEX root=../Main.tex
% \clearpage
\section{Appendix}

\subsubsection{Techniques for Better Generality}
\paragraph{The Higher spatiotemporal Sampling Training}
%插值方式选择
The Higher resolution and sampling rate generally improve model representations, leading to the better downstream performance. Instead of training on densely sampling inputs from stretch, we adopt a finetuning a high spatiotemporal sampling model from a low one as in \cite{wei2022masked} to cut down training costs. It initializes the model with the pretrained model at 224 resolution on our customized dataset, and then continues model training on the denser sampling inputs. Note the position encoding in the pretrained model needs to be adjusted to fit new spatiotemporal sampling specifics, otherwise the downstream performance would drop rapidly.
%As our model employs the 1D absolute position code generated with trigonometric function \cite{vaswani2017attention}, the easiest way to adjust it is to regenerate the code table based on the new input length. However, experiments have shown that this approach leads to performance degradation. 
We adopt 2D bicubic interpolation to implement spatial interpolation. When more frames as input is required, we used 1D linear interpolation in the time dimension while keeping the sampling interval. Note that using 3D trilinear interpolation directly in the spatiotemporal dimension performs almost identically to both using 2D and 1D interpolation in spatial and temporal dimension respectively.

% 超参调整参照convnet(warmup epoch, cutmix mixup), swin(min lr,调小weight decay), ours: drop path, base上repeat aug 关闭
When finetuning the model with a higher spatiotemporal sampling setting, it is necessary to tweak the previous hyper-parameter configuration for considering performance. 
%As the model already possesses a good initialisation at the time of finetune, keeping the previous finetuning hyperparameter settings will certainly introduce overfitting. 
Following \cite{liu2022convnet}, We turn off cutmix and mixup, and then ignore the warmup pharse with the minimal learning rate to $2e-7$ \cite{liu2021swin}. In particular, tuning the weight decay does not result in a significant performance change. To prevent overfitting, we reduce the learning rate by a factor of ten and the number of epochs by a factor of four. Note that turning up the drop path in the transformer block gives a significant performance boost as the resolution increases. To speed up model training and improve its stability, it is usual to perform repeated sampling \cite{Hoffer2020AugmentYB}. In practice, we do not employ this data augmentation in ViT models, except the model is Huge or larger.

%短边320 原视频会提升single view 但是multi-view会掉点 这可能是源于pretrain的数据来源不同
The different resolutions of the videos are obtained by directly resizing the samples in the dataset. The videos we use are already scaled to 320 on the short side while preserving their aspect ratios. Therefore, for higher resolutions (e.g. 384), we up-sample videos directly. Empirically, if we employ the original video data to finetune model, it will improve single-view testing performance at the cost of multi-view one. This may be caused by the various data sources used in pretraining and finetuning.
\paragraph{Data co-training}
\begin{figure}[t]
\centering
\includegraphics[width=0.5\textwidth]{content/figures/methods/cotrain.pdf}
\caption{\label{cotraining} \model~is training with single-label and multi-labels dataset in supervised video learning. Each dataset has individual task decoder and task-specific optimizer. \model~can jointly train all the tasks better when simply use tasks' hyper-parameters in single task training.}
\end{figure}
% 在传统的有监督学习范式下，网络在有限的domain中能够很快的学习到很好的表达。
Previous works [] show that video representation provided by masked reconstruction and multimodal matching could be further significantly improved on downstream application performance with supervised learning. Learning a representation using multiple tasks or datasets is called co-training []. Unlike our initial version Intern [] or Multiview Transformer [] leverages different tasks with the corresponding supervisions for training, we only tune video representation on one classification task (action recognition) with multiple datasets.
%Our initial version Intern frames its supervised training as multiple stages with different tasks, 

%\yinan{Masked video encoder and multi-modality contrastive modeling show good capabilities in transferring to video visual and text downstream tasks. It can quickly manifest strong empirical results in specific domain  when training by supervised datasets. Inspired by \cite{PolyViT,CoVeR}, we leverage different datasets to jointly learn a more general video representation.}

We employ a visual decoder composed of several classification heads to exploit different datasets. The used datasets include Kinetics~\cite{k400} and our annotated multi-label dataset. The backbone parameters and these of each head are updated with an independent AdamW~\cite{adamw} optimizer. Different datasets will be selected alternately in proportion to their total size.

For the optimization of co-training, we employ cross entropy loss for classical video classification with single labels. Since our self-collected and -annotated dataset is with multi-labels, we adopt the asymmetric loss~\cite{asl} to mitigate the long-tailed effect caused by extreme label imbalance in our multi-label datasets. Simply put, asymmetric loss~\cite{asl} is a multi-label version of focal loss [].

% 我们选取了多标签任务和单标签任务一起训练来丰富特征表示。每个数据集用一个优化器。 一个step只会有一个数据集，每个数据集轮番交替训练。
%\yinan{We choose multi-task training strategy and different dataset heads as decoder of visual encoder. To enrich the visual representation, we co-train the traditional dataset (i.e. Kinetics~\cite{k400}) with our annotated multi-labels dataset. In co-training strategy, we optimize the parameters of backbone and single decoder that we are co-training on with task-specific AdamW~\cite{adamw} optimizer. Data from only one dataset is fed into the model and optimized in one step. Different datasets will be selected alternately in proportion to their total data size. }

%\yinan{In single-label tasks, the parameters of encoder and decoder are simplely learnt by minimizing the cross entropy loss. To mitigating the effects of label imbalance in optimization process in multi-labels datasets, we adopt the asymmetric loss~\cite{asl} to dynamically down-weights and hard-thresholds easy samples and discarding possibly mislabeled samples.}

%
%\yinan{After co-training, model can encode various spatial feature and sufficient temporal information. Co-training multiple datasets can not only make single model processing different tasks at the same time but also lead model to learn a more robust representation.}

\subsection{Pretraining Data Curation}
Data used for pretraining are crucial guarantee for the effectiveness and generalization of the video foundation models. Our used data stem from two sources: public datasets and self-collected ones. Since \model~is consisted by masked video encoder and fused multi-modal one, the employed data are gathered in two manners due to the corresponding optimizations. 

We gather xx public datasets with action lables as a database for videoMAE training. Besides, we build a customized action dataset lasting no more than xx seconds from Instagram.

For multimodal learning, we employ webvid2M, xxx, along with self-built ones. Besides of video-language datasets, we also exploit image-text ones for between appearance-text alignment as in []. 

For subsequent supervised training, we find a superset of Kinetics (removing leaked data) works impressively compared with other trials. Specifically, we propose a unified video benchmark K710 for post-pretraining the used video encoders in supervised setting. 
\paragraph{Kinetics-710.} \label{k710}
We adopt a new customized kinetics action dataset Kinetics-710 \cite{uniformerv2} for supervised training, both separate and joint ones. It has 650K videos with 710 unique action labels. It combines all the unique training data from Kinetics 400/600/700~\cite{k400,k600,k700}. To avoid the training leak, some training data existing in the testing set from Kinetics of a specific version are abandoned.

%\subsubsection{Used Data}
%\paragraph{Public Data}
\bingkun{Kinetics, ssv2, ava, webvid2M, }
%\input{content/data/kinetics}

%\input{content/data/sthsth}

%\subparagraph{AVA\cite{gu2018ava}.}

%\subparagraph{webvid\cite{Bain21}.}

% 加描诉关于从instgram上下载的sta-web
\subsubsection{Self-collected Data}
% 大数据是大模型的基础
We collect video data and annotate some of them besides of the used public data. We find they are helpful to improve generality and downstream performance of VideoIntern.
%\yinan{Large-scale datasets are the cornerstone of many MML methods. Attributed to public video datasets, MAE and MML can get satisfactory visual representation. Further, video foundation model requires more comprehensive data distribution and richer text annotation. }
% 我们结合现有的公开数据集和ATUS合并了3.7k个标签词，组合成了query词，翻译成了10国语言，在Youtube上搜索，得到了1.2M的数据 -> 12M video clip

Based on the existing action labels from mainstream action datasets, we reorganize their relations and hierarchy using the semantic structure from U.S. time diary survey~\cite{atus}. More importantly, we extend the existing around 800 action labels (from Kinetics, something-something, moments, etc) into 3.7 thousand ones. All these labels are visible motion descriptions, exploited as the query phrases on the video websites for collecting relevent data. During collection, associative words and translation into other languages are enabled for getting videos from a broader and more diverse scenes and regions. Finally, we acquire around 1.2 million videos lasting from 15 minutes to 2 hours with 10 minute average length. Their audios and subtitles (if have) are also reserved, used for multi-modality learning.

%\yinan{From our point of improving the representation of motions, we collect action labels by aligning existing video datasets and the candidate words of U.S. time diary survey. We filter out 3.7k labels which is a phrase has a visible concept. We filter phrases that do not contain visual concepts (e.g. desire), leaving 3.7k phrases as the base vocabulary of the query items. We use the associative words of the search engine to augment our query words, keep the top ten recommended query items of each phrase, and translate them into 10 different languages through the translation toolkit. We collect 1.2 million videos with 37k query items from multiple sources. The videos contain an average of 10 minutes of sequence, audio. 10\% of them have user-generated subtitles, and about half of the videos contain ASR subtitles. These data form our video-text data pool.}

% \begin{figure}[t]
% \begin{center}
% \fbox{\rule{0pt}{2in} \rule{0.9\linewidth}{0pt}}
%   %\includegraphics[width=0.8\linewidth]{egfigure.eps}
% \end{center}
%   \caption{Placeholder. Statics of self-collected data.}
% \label{fig:self-collected-data}
% \end{figure}

\subsubsection{Data Sculpting}

% 对部分数据使用镜头切割得到小的片段，在使用CLIP打伪标签，再使用人工标注，得到multi-labels的有标注数据集

% 我们根据时间戳将长视频进行修剪，然后将片段的帧输入进经过大量图片-文本对训练的CLIP中，根据查询词获得最高的响应时间戳。我们将该帧的前后五秒作为一个视频序列再次输入到模型中，获得模型在3.7k个标签

Considering the collected videos are long and noisy, we develop a data sculpting pipeline upon public vision-language models to generate trimmed video clips for training. The basic idea is to extract clips highly correlated with our new action labels from videos.
We initially divide every original video into several segments based on frame differences. Then we localize the key frames in each segment and compute their semantic responses from CLIP~\cite{clip} in a prompt fashion, meaning computing the estimated likelihoods of all used labels with CLIP. Then we select top $n$ (we use $k=min(3,n)$ where $n$ denotes the number of keyframes in the segment) frames with the highest responses, and generate their corresponding clips by including a 10-second clip centering around them. Meanwhile, these clips are automatically annotated with pseudo labels from CLIP. For each clip, we preserve its top 4 labels with highest responses plus the original query one. 

%\yinan{To efficiency obtain the trimed video clips, we propose a simple self-collected data sculpting pipeline. 1) The timestamp of the shot is first calculated according to the change of the video frames. 2) We trim long videos based on timestamps and then feed the clips’ frames into CLIP~\cite{clip} trained on large-scale image-text pairs to get the highest response timestamps based on query phrases. 3) We feed this frame and the frames 5 seconds before and after it into the model as a sequence and obtain label candidates in 3.7k labels. }

For human annotation, we ask annotators to select all relevant labels from the given pseudo ones for each video clip, leading to a multi-label video action dataset. This dataset currently only has around 200 thousand clips with annotations.
% 讲的标注过程，感觉不一定需要。
%\yinan{In the process of human annotation, we ask workers to tell whether the top five labels output by the model exist in the current video clip. So we obtain multi-label video action annotations for model training.}

%\subsection{Downstream Applications}

% \end{method}

\subsection{Limitations}

\subsection{Experiments}
\subsubsection{Configuration}
\subsubsection{}
